# Supplementary material for: A Unified Approximation Framework for Compressing and Accelerating Deep Neural Networks
Source: arXiv:1807.10119 source file (2019-08-20)
Supplement: Supplementary file 1 [file appendix.tex]

{
\twocolumn[
\begin{@twocolumnfalse}
\begin{appendix}

\textbf{Appendix: ADMM update rules}:

\begin{align}
\bm{A}^{k+1} &= \underset{\bm{A}}{\textrm{argmin }} L_t(\bm{A},\bm{B}^k,\bm{M}^k;\bm{\Lambda}^k), \\
& = \underset{\bm{A}}{\textrm{argmin }}\lambda_1\norm{\bm{A}}_{2,1} + \langle \bm{\Lambda}^k, \bm{A}+\bm{B}^k-\bm{M}^k \rangle + \frac{t}{2}\norm{\bm{A}+\bm{B}^k-\bm{M}^k}_F^2 \\
& = \underset{\bm{A}}{\textrm{argmin }}\lambda_1\norm{\bm{A}}_{2,1} + \frac{t}{2}\norm{\bm{A}+\bm{B}^k-\bm{M}^k + \frac{\bm{\Lambda}^k}{t}}^2_F,
\end{align}
which is proximal operator of $l_{2,1}$ norm.

\begin{align}
\bm{B}^{k+1} &= \underset{\bm{B}}{\textrm{argmin }} L_t(\bm{A}^{k+1},\bm{B},\bm{M}^k;\bm{\Lambda}^k), \\
& = \underset{\bm{B}}{\textrm{argmin }}\lambda_2\norm{\bm{B}}_{*} + \langle \bm{\Lambda}^k, \bm{A}^{k+1}+\bm{B}-\bm{M}^k \rangle + \frac{t}{2}\norm{\bm{A}^{k+1}+\bm{B}-\bm{M}^k}_F^2 \\
& = \underset{\bm{B}}{\textrm{argmin }}\lambda_2\norm{\bm{B}}_{*} + \frac{t}{2}\norm{\bm{B}+\bm{A}^{k+1}-\bm{M}^k + \frac{\bm{\Lambda}^k}{t}}^2_F ,
\end{align}
which is proximal operator of nuclear-norm.

The update rules for $\bm{M}$ and $\bm{C}_n$ can be decided by first-order condition.
$\bm{C}_n$ can be derived through element-wise analysis.
\begin{equation}
\begin{aligned}
\bm{C}^{k+1}_n 
& =\underset{\bm{C}_n}{\textrm{argmin }}L_t(\bm{A}^k,\bm{B}^k,\bm{M}^k,\bm{C}^k_1 \cdots \bm{C}_n \cdots \bm{C}^k_N; \bm{\Lambda}_0^k \cdots \bm{\Lambda}_n^k) \\
& =\underset{\bm{C}_n}{\textrm{argmin }}\norm{\bm{Y}_n - r(\bm{C}_n)}_F^2 + \langle \bm{\Lambda}_n^k, \bm{M}^k\bm{X}_n - \bm{C}_n  \rangle + \frac{t}{2}\norm{\bm{M}^k\bm{X}_n - \bm{C}_n}_F^2.
\end{aligned}
\label{eq:admm2_c1}
\end{equation}

\begin{equation}
(\bm{C}^{k+1}_n)_{ij} = \left \{
\begin{aligned}
& \frac{t(\bm{M}^k\bm{X}_n)_{ij}+(\bm{\Lambda}_n^k)_{ij}+2(\bm{Y}_n^k)_{ij}}{2 + t}, && \textrm{ if } t(\bm{M}^k\bm{X}_n)_{ij}+(\bm{\Lambda}_n^k)_{ij} > -2(\bm{Y}_n^k)_{ij};  \\
& 0, && \textrm{ if } -2(\bm{Y}_n^k)_{ij} < t(\bm{M}^k\bm{X}_n)_{ij}+(\bm{\Lambda}_n^k)_{ij} < 0; \\
& \frac{t(\bm{M}^k\bm{X}_n)_{ij}+(\bm{\Lambda}_n^k)_{ij}}{t}, && \textrm{ if } t(\bm{M}^k\bm{X}_n)_{ij}+(\bm{\Lambda}_n^k)_{ij} < -2(\bm{Y}_n^k)_{ij}.
\end{aligned}
\right .
\end{equation}
\label{eq:admm2_c2}

$\bm{M}$ can be derived by solving a matrix equation.
\begin{equation}
\begin{aligned}
\bm{M}^{k+1} &= \underset{\bm{M}}{\textrm{argmin }}L_t(\bm{A}^k,\bm{B}^k,\bm{M},\bm{C}^k_1 \cdots \bm{C}^k_N; \bm{\Lambda}_0^k \cdots \bm{\Lambda}_n^k) \\
&= \underset{\bm{M}}{\textrm{argmin }} \langle \bm{\Lambda}_0^k, \bm{A}^k+\bm{B}^k-\bm{M} \rangle + \frac{t}{2}\norm{\bm{A}^k+\bm{B}^k-\bm{M}}_F^2 +  \sum_{n=1}^{N}\langle \bm{\Lambda}_n^k, \bm{M}\bm{X}_n - \bm{C}_n^k  \rangle + \sum_{n=1}^{N}\frac{t}{2}\norm{\bm{M}\bm{X}_n - \bm{C}_n^k }_F^2
\end{aligned}
\label{eq:admm2_m1}
\end{equation}

\begin{equation}
\textrm{Set gradient to be 0}\Rightarrow \partial_ML_t = -\bm{\Lambda}_0^k - t(\bm{A}^k+\bm{B}^k-\bm{M}) + \sum_{n=1}^{N}t(\bm{M}\bm{X}_n-\bm{C}_n^k)\bm{X}_n^T + \sum_{n=1}^{N}\bm{\Lambda}_n^k\bm{X}_n^T = \bm{0}.
\end{equation}

\begin{equation}
\Rightarrow t\bm{M}(\bm{I}+\sum_{n=1}^{N}\bm{X}_n\bm{X}_n^T) = \sum_{n=1}^{N}(t\bm{C}_n^k\bm{X}_n^T-\bm{\Lambda}_n^k\bm{X}_n^T) + t(\bm{A}^k + \bm{B}^k) + \bm{\Lambda}_0^k
\label{eq:admm2_m2}
\end{equation}

\end{appendix}
\end{@twocolumnfalse}
]
